# Supplementary material for: Revisiting Multi-User Downlink in IEEE 802.11ax: A Designers Guide to MU-MIMO
Source: arXiv:2406.05913 source file (2024-08-19)
Supplement: Supplementary file 1 [file appendix.tex]

\subsection{Appendix 1}\label{app:1}
